# Supplementary material for: Learning to Build by Building Your Own Instructions
Source: arXiv:2410.01111 source file (2024-10-01)
Supplement: Supplementary file 1 [file supplemental.tex]

\documentclass[runningheads]{llncs}

% ---------------------------------------------------------------
% Include basic ECCV package
 
% TODO REVIEW: Insert your submission number below by replacing '*****'
% TODO FINAL: Comment out the following line for the camera-ready version
%\usepackage[review,year=2024,ID=12536]{eccv}
% TODO FINAL: Un-comment the following line for the camera-ready version
\usepackage{eccv}

% OPTIONAL: Un-comment the following line for a version which is easier to read
% on small portrait-orientation screens (e.g., mobile phones, or beside other windows)
%\usepackage[mobile]{eccv}

% ---------------------------------------------------------------
% Other packages

% Commonly used abbreviations (\eg, \ie, \etc, \cf, \etal, etc.)
\usepackage{eccvabbrv}

% Include other packages here, before hyperref.
\usepackage{graphicx}
\usepackage{booktabs}

\usepackage{tabularx}
\usepackage{algorithm}
\usepackage[noend]{algpseudocode}

% The "axessiblity" package can be found at: https://ctan.org/pkg/axessibility?lang=en
\usepackage[accsupp]{axessibility}  % Improves PDF readability for those with disabilities.

% ---------------------------------------------------------------
% Hyperref package

% It is strongly recommended to use hyperref, especially for the review version.
% Please disable hyperref *only* if you encounter grave issues.
% hyperref with option pagebackref eases the reviewers' job, but should be disabled for the final version.
%
% If you comment hyperref and then uncomment it, you should delete
% main.aux before re-running LaTeX.
% (Or just hit 'q' on the first LaTeX run, let it finish, and you
%  should be clear).

% TODO FINAL: Comment out the following line for the camera-ready version
%\usepackage[pagebackref,breaklinks,colorlinks,citecolor=eccvblue]{hyperref}
% TODO FINAL: Un-comment the following line for the camera-ready version
\usepackage{hyperref}

% Support for ORCID icon
\usepackage{orcidlink}

\begin{document}

\newcommand{\rcvehicles}{RC-Vehicles}
\newcommand{\ours}{InstructioNet}

%\maketitle
%\input{sections/abstract}    
%\input{sections/introduction}
%\input{sections/related_work}
%\input{sections/method}
%\input{sections/experiments}
%\input{sections/conclusion}
%{
%    \small
%    \bibliographystyle{ieeenat_fullname}
%    \bibliography{main}
%}

% WARNING: do not forget to delete the supplementary pages from your submission 
%\newpage
\appendix
\input{appendices/additional_ablations}
\input{appendices/expert_details}
\input{appendices/training_algorithm}

\end{document}
